# Supplementary material for: Sub-laser-cycle control of relativistic plasma mirrors
Source: arXiv:2107.13888 source file (2021-07-29)
Supplement: Supplementary file 1 [file Supplement.pdf]

# Supplementary Information to
# *Sub-laser-cycle control of relativistic plasma mirrors*

L. Chopineau,[1,2] G. Blaclard,[1] A. Denoeud,[1,2] H. Vincenti,[1] F. Quéré,[1] and S. Haessler[3]

[1]*LIDYL, CEA, CNRS, Université Paris-Saclay, CEA Saclay, 91191 Gif-sur-Yvette, France*
[2]*CEA, DAM, Bruyères-le-Châtel, 91297 Arpajon*
[3]*Laboratoire d'Optique Appliquée, Institut Polytechnique de Paris, ENSTA-Paris, Ecole Polytechnique, CNRS, 91120 Palaiseau, France*

(Dated: July 29, 2021)

## I. EXPERIMENTAL SETUP

The experiments are carried out on UHI100, the 100 TW-class Ti:sapphire laser facility at LIDYL (CEA Saclay), delivering 25-fs pulses at central wavelength $\lambda = 800\,\text{nm}$. An extremely high temporal contrast ratio of $\gtrsim 10^{13}$ on a $\gtrsim 100$ ps timescale is achieved thanks to a double plasma-mirror setup [1]. In these conditions, the maximum energy on target is $\sim 0.5\,\text{J}$, distributed in a 65-mm-diameter near-top-hat beam. A deformable mirror coupled to a wavefront sensor (Imagine Optic) corrects aberrations thus optimizing the focal spot on target.

The optical setup preparing the pulse sequence sent on target is shown on Fig. SM1. The scale length $L_g$ of the plasma density gradient, $n(x) \propto \exp[x/L_g(\tau)]$ is controlled by a weak prepulse ($F \simeq 10^3$ J/cm$^2$ on target) at an adjustable delay $\tau$ before the main beam [2]. Its value was measured using spatial domain interferometry [3]. An aperture mask then transmits the prepulse as well as a 33-mm-diameter top-hat main beam (limited by the available size of the calcite crystal mentioned below).

The two-color waveforms are generated by a combination of three transmissive optics [4, 5]: part of the fundamental light with frequency $\omega_L$ is frequency-doubled to $2\omega_L$ in an 800-$\mu$m thick KDP crystal ($C_1$; Gooch & Housego), which can be rotated away from the optimum phase-matching angle to reduce the conversion efficiency from its maximum of $\approx 25\%$ down to zero. Due to the top-hat beam profile we suppose a spatially uniform SHG efficiency. The temporal walkoff due to dispersion is partly compensated by shortening due to the nonlinearity of SHG [5] so that we suppose a 35-fs pulse duration for the $2\omega$-component.

The timing of the two color-components is controlled by a 1.5-mm thick calcite crystal ($C_2$; 35 mm$\times$35 mm; Berhard Halle Nachfl.) with its optic axis oriented at 45° to the crystal front surface and perpedicular to the fundamental's polarization axis. As shown in Fig. SM2, small rotations of the crystal about this axis lead to quasi-linear shifts of the relative group delay $\tau_g$ and phase delay $\tau_\phi$ of the two color components. Their temporal pulse envelopes are well

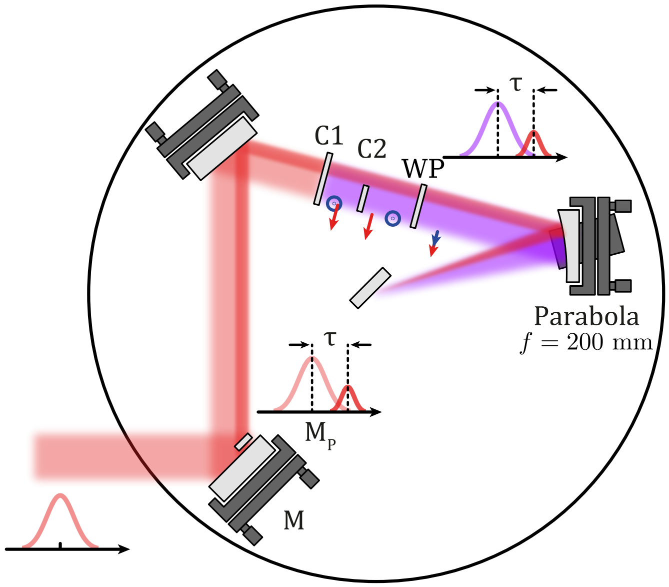


FIG. SM1. **Optical experimental setup** with the prepulse (red) and main pulse (purple) with adjustable relative delay $\tau$ as set by the two-part mirror M / $M_P$, and the three crystals $C_1$, $C_2$, WP for two-color waveform generation (see text).

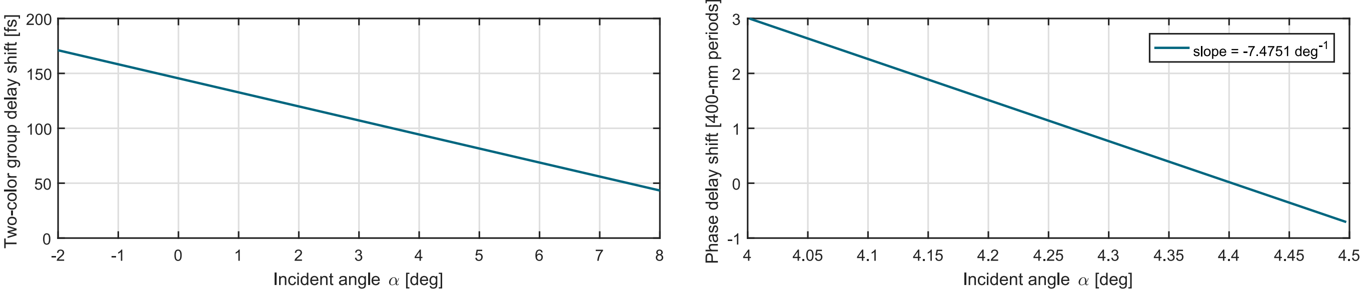


FIG. SM2. **Timing control through the calcite-plate (C2) orientation.** Calculated relative group (left) and phase delays (right) between the 800-nm fundamental and the 400-nm second harmonic as a function of the incidence angle on the birefringent calcite crystal.

overlapped for a 4.3° incidence angle on the calcite crystal as the $\tau_{\rm g} \approx 90$ fs group delay induced by the propagation through the KDP (C1) and subsequent waveplate (WP) are compensated. Scanning the calcite angle in small steps ($\sim 0.01°$) over a 0.13°-wide range around this position shifts the group delay in total by $\approx 1.7$ fs and the phase delay by $\tau_\phi = 1.34$ fs, the latter corresponding to $T' = 2\pi/2\omega_L$, i.e. one period of the second harmonic. Such a scan therefore covers the full range of two-color optical-cycle shapes with excellent temporal stability and reproducibility while keeping the pulse envelopes well overlapped. Finally, a 273-$mu$m thick quartz wave plate (WP; 6.5$\lambda$400 nm, 3$\lambda$800 nm; Eksma Optics) rotates the polarization direction of the second harmonic so as to be parallel to that of the fundamental. The total energy of the two-color pulses on target is $\approx 125$ mJ.

## II. ADDITIONAL EXPERIMENTAL RESULTS

### A. Gradient scale length dependence with $\omega_{\rm L}$-single-color driver

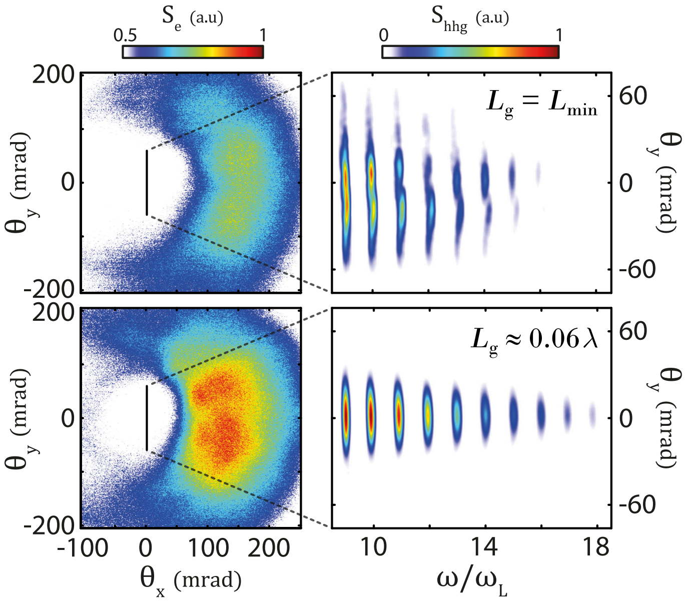


FIG. SM3. **Gradient scale length $L_{\rm g}$ dependence of HHG and electron emission with a single-color ($\omega_{\rm L}$) driver.** Angular emission pattern of accelerated electrons (left column) and angularly-resolved harmonic spectrum (right column) obtained with the minimal gradient scale length (upper row) and with a gradient scale length optimizing both ROM HHG and vaccum-laser-accelerated electron emission. The vertical black lines in the electron beam profiles mark the XUV spectrometer angular acceptance.

We performed a scan of the plasma gradient scale length $L_{\rm g}$ for a single-color main beam. As shown in Fig.SM3, in our moderately relativistic driving intensity, we find the same behavior as reported earlier for higher intensities [2,

6]. The steepest experimentally accessible gradient, $L \lesssim \lambda/50$, strongly favors the coherent-wake-emission (CWE) process [7] for HHG, with its associated rather high divergence and marked spatial modulations of the emitted beam. A scale length $L \approx \lambda/16$ provides optimal conditions for the relativistic oscillating mirror (ROM) process [2, 6, 8], which at moderately relativistic driving intensities leads to lower-divergence spatially smooth beams [2, 9]. Fig.SM3 shows this striking spatial difference in the measured HHG spectra, evidencing the transition from a dominance of CWE to ROM harmonics despite the absence of signal beyond the CWE spectral cutoff. The resemblance to the angle-resolved HHG spectra shown in Fig.2 of the main manuscript or in the upper row of Fig. SM4 strongly supports our interpretation that in the scan of the phase-delay $\tau_\phi$ characterizing the two-color driving waveforms, we observe an on-off oscillation of ROM HHG on top of a CWE background.

Detecting the electron spatial distribution in such scans we find a correlation of the ejected charge with the ROM efficiency, i.e. a maximum for $L \approx \lambda/15$. Both the ROM mechanism and electron acceleration benefit from the charge separation field produced at longer gradients. Their correlation for sinusoidal, i.e. single-color, driving waveforms has been reported earlier [6] and interpreted in the framework of the push-pull model [10].

### B. Gradient scale length dependence with $\omega_\mathrm{L} + 2\omega_\mathrm{L}$ two-color driver

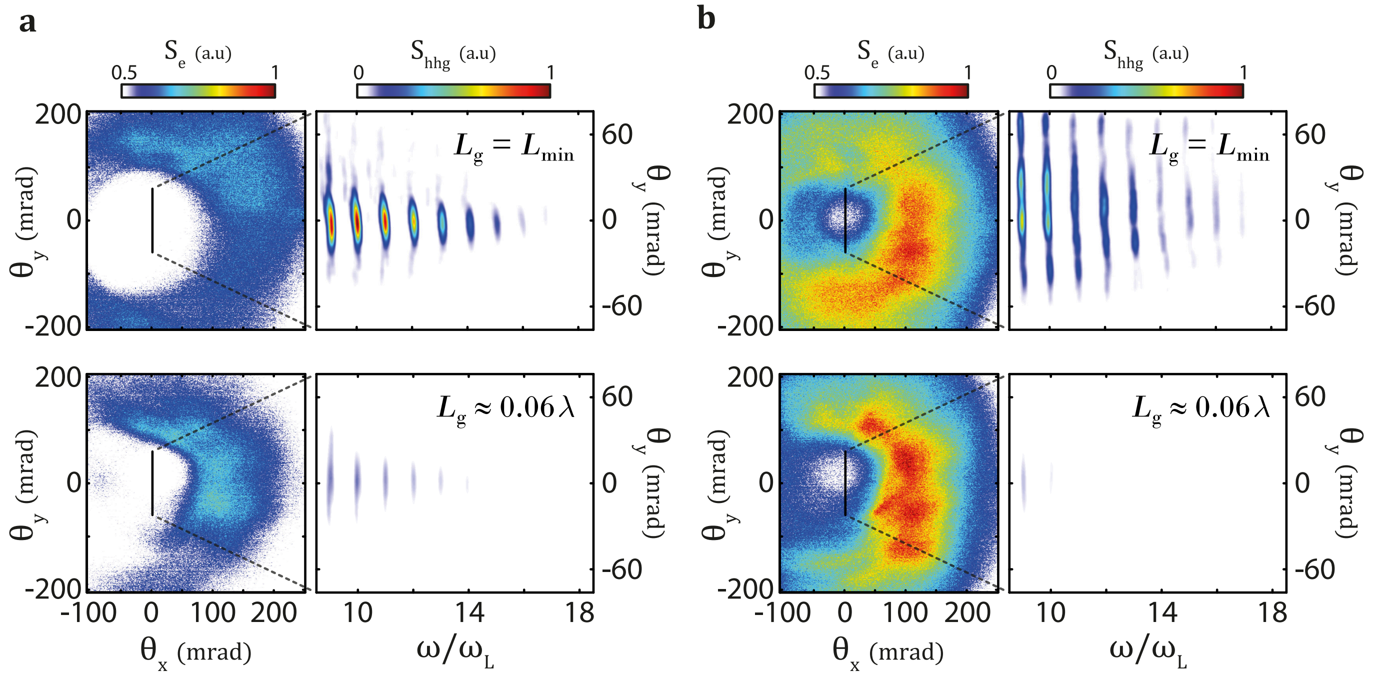


FIG. SM4. **Gradient scale length $L_\mathrm{g}$ dependence of HHG and electron emission with a two-color ($\omega_\mathrm{L} + 2\omega_\mathrm{L}$) driver.** Angular emission pattern of accelerated electrons (left) and angularly-resolved harmonic spectrum (right) obtained with the same two gradient scale lengths as in Fig.SM3 ($L_\mathrm{g} \approx 0$ above and $L_\mathrm{g} \approx \lambda/16$ below). The phase delay of the two-color driving waveforms is set such that it optimizes low-divergence ROM HHG emission (**a**) or fast electron emission (**b**). The vertical black lines in the electron beam profiles mark the XUV spectrometer angular acceptance.

Figure SM4 shows HHG spectra and electron beam profiles measured with $\omega_\mathrm{L} + 2\omega_\mathrm{L}$ two-color driving waveforms with the phase delays $\tau_\phi$ set so as to either optimize low-divergence ROM HHG emission (left column) or electron emission (right column). For each driving waveform, the plasma gradient scale length $L_\mathrm{g}$ was scanned. Figure SM4 shows the data for the same two scale lengths as in Fig. SM3, i.e. the shortest accessible value $L_\mathrm{g} \leq \lambda/50$ as well as $L_\mathrm{g} \approx \lambda/16$, found optimal for *both* ROM HHG and electron emission with the $\omega_L$-single-color driver (cf. Fig. SM3).

Here, with both two-color driving waveforms, we find that while the ejected electron charge barely changes when increasing $L_\mathrm{g}$ up to $\approx \lambda/16$, the HHG signal rapidly drops and has almost completely vanished for the scale length $L_\mathrm{g} \approx \lambda/16$. Thus, the effect of the plasma density gradient scale length is different for single-color and two-color driving waveforms, and there is thus no longer a common set of optimal conditions for HHG and electron emissions in the two-color case.

## III. PIC SIMULATIONS

The simulations presented in the paper were performed with the Particle-In-Cell code WARP+PXR that relies on a very accurate pseudo-spectral solver – PSATD (Pseudo-Spectral Analytic Time Domain) – where the fields are analytically integrated in Fourier space over a finite time step. The advantage of such a solver is that it largely mitigates most numerical effects; in particular it suppresses all effects related to numerical dispersion, present in all finite-difference based solvers. It then allows for a better convergence to the solution in term of computational resources.

In table I, we summarize the numerical and physical parameters used for our 1D and 2D simulations. Note that the 1D simulations were performed in a Lorentz boosted frame to emulate an angle of incidence $\theta$ of the laser on target.

| | 1D | 2D |
|---|---|---|
| Maxwell solver | PSATD | PSATD |
| $\Delta x$ ($\Delta y$) | $\lambda/350$ | $\lambda/160$ |
| $c\Delta t$ | $\Delta x$ | $\Delta x$ |
| nb part/cell | 500 | $5 \times 5$ |
| $a_0$ ($\omega_L$) | 1 | 1 |
| $a_0$ ($2\omega_L$) | 0.5 | 0.5 |
| Laser duration | $\sim$ 30fs | $\sim$ 30fs |
| Target density | 220 $n_c$ | 220 $n_c$ |
| $L$ | $\lambda$ / 50 | $\lambda$ / 50 |
| $\theta$ | 55° | 55° |
| $\tau_\phi$ | $nT_L/16$ | $nT_L/16$ |

TABLE I. **Numerical and physical parameters for simulations presented in the paper.** Here, $\theta$ is the angle of incidence, $\Delta x$ and $\Delta y$ the spatial steps, $\Delta t$ the temporal step, $c$ the celerity of light and $n$ is an index to tune to modify the delay between the two color components.


[1] A. Lévy *et al.*, Optics Letters **32**, 310 (2007).
[2] S. Kahaly *et al.*, Physical Review Letters **110**, 175001 (2013).
[3] M. Bocoum *et al.*, Optics Letters **40**, 3009 (2015).
[4] N. Dudovich *et al.*, Nature Physics **2**, 781 (2006).
[5] M. Yeung *et al.*, Nature Photonics **11**, 32 (2017).
[6] L. Chopineau *et al.*, Physical Review X **9**, 011050 (2019).
[7] F. Quéré *et al.*, Physical Review Letters **96**, 125004 (2006).
[8] C. Rödel *et al.*, Physical Review Letters **109**, 125002 (2012).
[9] B. Dromey *et al.*, Nature Physics **5**, 146 (2009).
[10] M. Thévenet, H. Vincenti, and J. Faure, Physics of Plasmas **23**, 063119 (2016).
